# Supplementary material for: Do I Need the Cloud? Uncertainty-Aware Step-Level Handoff for Small Language Model Agents
Source: arXiv:2610.07816 source file (2026-10-06)
Supplement: Supplementary file 1 [file appendix_models_filled.tex]

\begin{table}[h]
\centering\small
\caption{Per-model results at 30\% fixed cloud budget, real BFCL subset. Three local/strong pairs were evaluated (a single strong model and three SLM sizes).}
\label{tab:appendix_models}
\begin{tabular}{lccccc}
\toprule
Local / strong pair & Params & Task succ. & Cloud \% & Risky errors & Latency\\
\midrule
qwen2.5-0.5b / qwen2.5-7b & 0.5B & 73.1 & 26.9 & 3.8 & 0.351\\
qwen2.5-1.5b / qwen2.5-7b & 1.5B & 82.7 & 30.8 & 3.8 & 0.777\\
qwen2.5-3b / qwen2.5-7b & 3B & 90.4 & 26.9 & 3.8 & 1.153\\
\bottomrule
\end{tabular}
\end{table}
