# Supplementary material for: Do I Need the Cloud? Uncertainty-Aware Step-Level Handoff for Small Language Model Agents
Source: arXiv:2610.07816 source file (2026-10-06)
Supplement: Supplementary file 2 [file appendix_shift_filled.tex]

\begin{table}[h]
\centering\small
\caption{Distribution-shift evaluation: NOT RUN this session. The shifted evaluation splits (unseen tool families, paraphrased schemas, additional distractor tools, longer trajectories) were not constructed -- doing so honestly requires new held-out BFCL-derived splits with verified shift properties, which was out of scope for the available compute/time budget (see reproducibility\_report.md). All cells are marked N/A rather than estimated or extrapolated from the in-distribution result; this table is left as a documented, explicit gap for future work.}
\label{tab:appendix_shift}
\resizebox{\linewidth}{!}{%
\begin{tabular}{lcccc}
\toprule
Shift & SLM only & Query router & \method & Strong only\\
\midrule
In-distribution$^\dagger$ & N/A & N/A & N/A & N/A\\
Unseen tool families & N/A & N/A & N/A & N/A\\
Paraphrased schemas & N/A & N/A & N/A & N/A\\
More distractor tools & N/A & N/A & N/A & N/A\\
Longer trajectories & N/A & N/A & N/A & N/A\\
\bottomrule
\end{tabular}%
}
\end{table}
